# Supplementary material for: Dark energy: EFTs and supergravity
Source: arXiv:2208.00177 source file (2022-07-30)
Supplement: Supplementary file 1 [file gbds_details.tex]

\chapter{Some explicit results for the quadratic curvature corrections}

\section{Coefficients of the leading order correction in the GB coupling expansion}\label{app:coeffs}
\begin{align}
    A_{n,p}&= 4n(p-7)(1-p) + 4n^2(1-p) + 4p(p-11) + 48 \ ,
    \\
    B_{n,p}&= -4\left[(n - 1)p^2 + (n^2 - 4n + 3)p - n^2 + 3n\right](p - 1)\ ,
    \\
    C_{n,p}&= 8\left[(n -1 )p^3 + (n^2 -11n + 14)p^2 - (2n^2 - 19n + 27)p + n^2 - 7n + 12\right]\ ,
    \\
    D_{n,p}&= 8(p- n)(np - n - p + 3)(p - 1)\ ,
    \\
    E_{n,p}&=4\left[2(3n - 5)p^3 - (2n^2 + 15n - 31)p^2 + (3n^2 + 12n - 31)p + n^2 - 7n + 12\right],
    \\
    F_{n,p}&=4(p - 1)(4n^2p^2 - 7n^2p - 7np^2 + n^2 + 14np + p^2 - 3n - 3p)\ .
\end{align}

\section{Field equations}
\label{sec:fieldeqs}

The $D$-dimensional field equations associated with \eqref{eq:action} read:
\begin{align}
	\begin{split}
		\label{eq:EinsteinD}
		0&=f(\varphi)\left(4R_A^{~C}R_{BC}+\dfrac12\mathcal{G}g_{AB}-2RR_{AB}+4R^{CD}R_{ACBD}-2R_A^{~CDE}R_{BCDE}\right)
		\\
		&\quad+\dfrac12\nabla_A\varphi\nabla_B\varphi-\dfrac14(\nabla\varphi)^2g_{AB}+2f'(\varphi)\left(R\,\nabla_A\nabla_B\varphi-4R_{(B}^{~C}\nabla_{A)}\nabla_C\varphi+2G_{AB}\Box\varphi\right.
		\\
		&\quad+2g_{AB}R^{CD}\nabla_C\nabla_D\varphi-2R_{ACBD}\nabla^C\nabla^D\varphi\left.\right)+2f''(\varphi)\left[R\,\nabla_A\varphi\nabla_B\varphi\right.\vphantom{\dfrac12}
		\\
		&\quad\left.-4R_{C(B}\nabla_{A)}\varphi\nabla^C\varphi+2G_{AB}(\nabla\varphi)^2+2g_{AB}R^{CD}\nabla_B\varphi\nabla_C\varphi-2R_{ACBD}\nabla^C\varphi\nabla^D\varphi\right] \vphantom{\dfrac12}
		\\
		&\quad-\dfrac{1}{2\kappa_D^2}G_{AB}-g(\varphi)\left[\dfrac{1}{2k!}H_{A_1...A_k}H^{A_1...A_k}g_{AB}-\dfrac{1}{(k-1)!}H_{A_1...A_{k-1}A}H^{A_1...A_{k-1}}_{~~~~~~~~~B}\right]
		\\
		&\quad-\dfrac12V(\varphi)g_{AB},
	\end{split}
	\\
	0&=\Box\varphi+f'(\varphi)\mathcal{G}-V'(\varphi)-\dfrac{g'(\varphi)}{k!}H_{A_1...A_k}H^{A_1...A_k},
	\label{eq:scalD}
	\\
	0&=\nabla_B\left[g(\varphi)H^{A_1...A_{k-1}B}\right].
	\label{eq:topform}
\end{align}
